# Supplementary material for: First-principles study of the energetics and the local chemical ordering of tungsten-based alloys
Source: arXiv:2410.03998 source file (2024-10-12)
Supplement: Supplementary file 1 [file Appendix_properties_alloying_elements.tex]

\section{SRO values of W-based alloys}
\label{SRO_values_w_alloys}

\begin{landscape}
\begin{table}[hbtp!]
\caption{\label{table_transmute_after_10years}{SRO values of W-alloys after Monte Carlo coupled DFT calculation in the nearest neighbor, the second nearest neighbor, and their average.}}
\vspace{2mm}
\centering
\begin{tabular}{c|cccccccccccc}
%\hline
\toprule
\multicolumn{1}{c}{Material} & \multicolumn{3}{c}{HEA1} & \multicolumn{3}{c}{HEA2} & \multicolumn{3}{c}{SA1} & \multicolumn{3}{c}{SA2} \\
% Material &W & SA1 & SA2 & HEA1 & HEA2  \\
% \cline{1-1}Element\\
\hline%\vspace{-7mm}\\
Pairs &  First & Second & Average & First & Second & Average & First & Second & Average & First & Second & Average \\
W-W & 0.003 & 0.125 & 0.071 & 0.437 & 0.333 & 0.393 & 0.113 & -0.125 & 0.011 & 0.169 & -0.292 & -0.029 \\
W-Ti & -0.188 & -0.313 & -0.241 & -0.158 & -0.333 & -0.233 & 0.186 & -0.488 & -0.103  & -- & --& --\\
W-Ta  & -0.125 & 0.188 & 0.009 & -0.359 & 0.271 & -0.089  & --& --& -- & --& --& --\\
W-Cr  & 0.281 & 0.008 & 0.161 & - & - & - &-0.329 & 0.441 & -0.0037  & -0.414 & 0.640 & 0.038 \\
Ti-Ti  & 0.128 & 0.330 & 0.214 & 0.104 & 0.619 & 0.325  & 1  & 1 & 1 & --& --& -- \\
Ti-Ta  & 0.284 & -0.193 & 0.079 & 0.259 & -0.545 & -0.086 & --  & --  & -- & --& --& --\\
Ti-Cr   & -0.230 & 0.183  & -0.053 & - & - & - & -0.706 & 1 & 0.025 & --& --& --\\
Ta-Ta  &  0.812 & -0.782 & 0.129 & 0.595 & -0.131 & 0.284  & -- & -- & -- & --& --& --\\
Ta-Cr  &  -0.961  & 0.772 & -0.218 & - & - & --& --& -- & -- & --& --& --\\
Cr-Cr   & 0.906 & -0.958 & 0.107 & - & - & - & 1 & -1.325 & 0.003  & 1 & -1.427 & -0.04 \\
W-V  & 0.053 & -0.190 & -0.051  & 0.094 & -0.291 & -0.071 & --   & --   & -- & --& --& --\\
Ti-V  & -- & -- & --  & -0.204 & 0.259 & -0.006 & --& --  & -- & --& -- & --\\
V-V  & -- & --  & -- & 0.625 & -0.375 & 0.196 & -- & --& -- & -- & --& --\\
V-Ta & -- & -- & --& -0.5 & 0.396 & -0.116 & --& --& --& --& --& --\\
W-Y   &  --  & -- & -- & -- & -- & --  & --& --& -- & 1 & -0.240 & 0.468 \\
Cr-Y  & --  & -- & --& -- & -- & --  & --& --& --  & -2.2 & 1 & -0.829 \\
Y-Y  & -- & -- & -- & -- & -- & -- & --& --& --  & 1 & -3.571 & -9.667\\
%\hline
\bottomrule
\end{tabular}
\end{table}
\end{landscape}
